# Supplementary material for: Path-encoded high-dimensional quantum communication over a 2 km multicore fiber
Source: arXiv:2103.05992 source file (2021-03-10)
Supplement: Supplementary file 1 [file SI.pdf]

# Supplementary Information

## Path-encoded high-dimensional quantum communication over 2 km multicore fiber

Beatrice Da Lio[1], Daniele Cozzolino[1], Nicola Biagi[2], Yunhong Ding[1], Karsten Rottwitt[1], Alessandro Zavatta[2,3], Davide Bacco[1*], Leif K. Oxenløwe[1]

[1] *Center for Silicon Photonics for Optical Communication (SPOC), Department of Photonics Engineering, Technical University of Denmark, 2800 Kgs. Lyngby, Denmark.*
[2] *CNR - Istituto Nazionale di Ottica (CNR-INO), Largo E. Fermi, 6 - 50125 Firenze, Italy.*
[3] *LENS and Dipartimento di Fisica e Astronomia, Università di Firenze, Via G. Sansone, 1 - 50019 Sesto Fiorentino, Italy.*
**dabac@fotonik.dtu.dk*

## Supplementary Note 1: Phase-locked loop details

The faithful transmission of quantum states on multicore fibers requires a phase-locked loop (PLL), that is a stabilization system that tracks and compensates for phase drifts. Such a system is implemented by an electronic board that uses the detected events from a single photon detector, placed in one output of the interferometer, as reference signal ($RS$), and gives as output an electric signal driving a phase actuator [1], in our case a phase shifter. The locking algorithm implemented on the board is constituted by the *scanning* and the *active locking* parts. In the scanning part, the reference signal is measured by an analog-to-digital converter of an ADUC7020 micro-controller, while a linear voltage ramp is applied to the phase actuator to produce a phase scan of $2\pi$. In this way, the maximum ($M$) and minimum ($m$) values of the reference signal are identified. Given these parameters, it is possible to determine the value of the reference signal corresponding to a precise phase value $\tilde{\varphi}$ by the equation:

$$RS(\tilde{\varphi}) = \frac{M+m}{2} + \frac{M-m}{2}\cos(\tilde{\varphi}) \tag{S1}$$

The active locking part of the algorithm is a digital implementation of a proportional-integral-derivative controller, in which the value $RS(\tilde{\varphi})$ is used as set point, *i.e.* as locking point. During this process, the reference signal is continuously monitored and the voltage applied to the phase actuator is changed to keep the reference signal as close as possible to the set point $RS(\tilde{\varphi})$.
The PLL boards used in our demonstration require an input reference signal that spans from 0.5 to 2 V to ensure correct locking conditions. The input signal can be amplified, with a limited gain, to reach this condition. In our setup, this translates into having count rates from the stabilisation channel detectors in the order of 150-200 kHz in the condition of constructive interference. Hence, the optimal condition for a stable locking was obtained by setting our InGaAs single photon avalanche detectors with 5 $\mu$s dead time, leading to a maximum count rate of 200 kHz, and 15% efficiency. Moreover, the optical power launched in the stabilization channel was checked using the same detectors while blocking one interferometer arm at the time and setting the count rate to approximately 80 kHz.
In this configuration, thanks to the wavelength division multiplexing filters introduced in the setup, the leakage from the stabilization channel to the SNSPDs used to detect the quantum states was limited to less than 10 kHz per detector. Being the actual count rates from the quantum communication channel in the order of tens of MHz per detector (for a fiber propagation loss of 5.8 dB), the leakage from the stabilization channel is then irrelevant and does not increase the overall QBER.

## Supplementary Note 2: System stability

In order to test the long term stability of our system, we have measured the QBER of one of the two MUBs ($\mathcal{X}$ basis). In this measurement, the system runs automatically without any external interference. The measurement reported in Figure 1 is acquired during an entire afternoon, from 1 pm to 9 pm. Our system is able to guarantee a positive QBER (below the coherent threshold) for more than 7 hours. Subsequently, the system slowly drifts and the QBER increases. There are different reasons for this behavior that can stem from polarization changing due to the temperature fluctuation in the room and to the fiber instability.

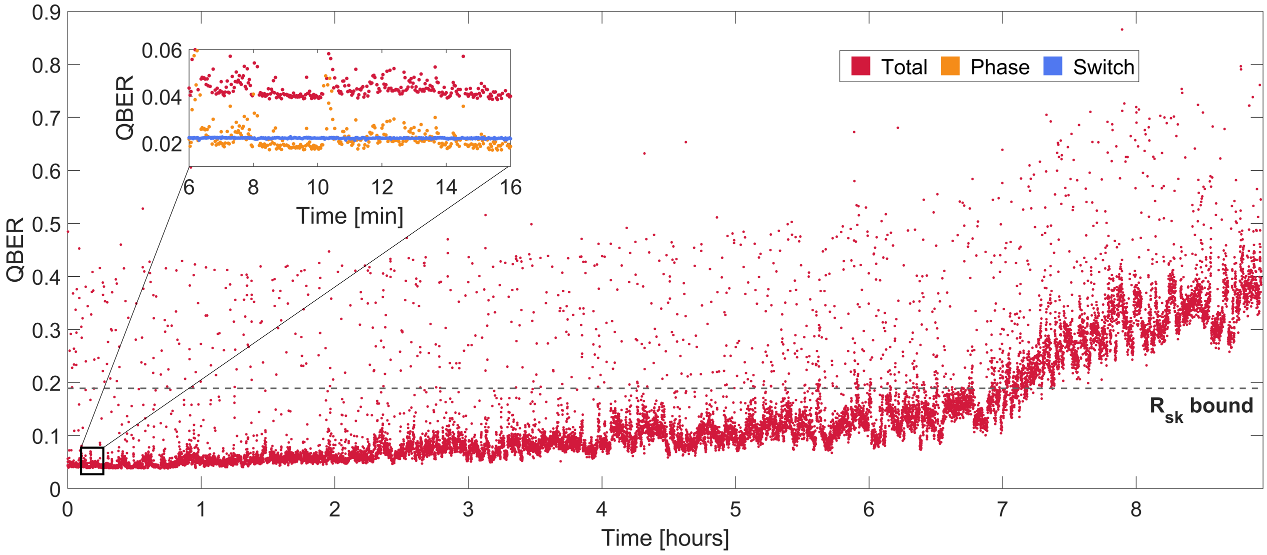


**Supplementary Figure 1: Long term system stability.** Measured QBER in the $\mathcal{X}$ basis over more than 8 hours of continuous acquisition. Data above the main trend show moments when the tracking system lost its locking position, yet recovering right away the previous stable QBER value. The inset shows a magnification of the same acquisition from minute 6 to 16: in red, the total QBER measured, and in orange and blue its two contributions due to errors in the phase modulation and stabilization, and to the switch modulation respectively. The dashed line shows the coherent attack threshold.

## Supplementary Note 3: Towards a complete QKD system based on multicore fibers

In this section, we propose the design of a possible setup able to actively choose between the two bases in Eq. (1) of the manuscript. As shown in figure 2, after the generation of weak coherent pulses (WCPs), a first optical switch operates the basis selection, sending the light to other two switches that will prepare the quantum states. After each of the last two optical switches, the same experimental setup presented in the manuscript is needed. However, in this case two different stabilization channels at $\lambda_1$ and $\lambda_2$ are required: one for each basis. After the transmission through a multicore fiber (MCF), the quantum states are detected using the same scheme used in our experiment for each basis.

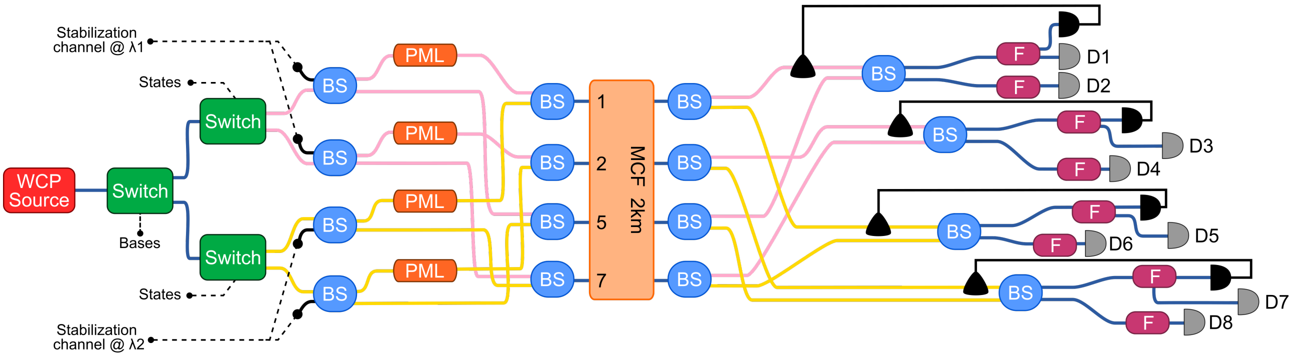


**Supplementary Figure 2: Full system setup.** WCP: weak coherent pulses; Switch: optical switch; BS: beam splitter; PML: phase modulation loop, see figure 2 a); MCF: multicore fiber; black triangle: phase shifter; F: wavelength division multiplexing filters; D1 to D8: superconducting nanowire single photon detectors; black detectors: InGaAs single photon detectors.

## Supplementary References


[1] N. Biagi, L. Costanzo, M. Bellini and A. Zavatta, "Entangling macroscopic light states by delocalized photon addition," *Phys. Rev. Lett.*, vol. 124, no.3, p. 033604, 2020.
